# Supplementary material for: No evidence for a strong decrease of planetesimal accretion in old white dwarfs
Source: arXiv:2111.12152 ancillary file (2021-11-23)

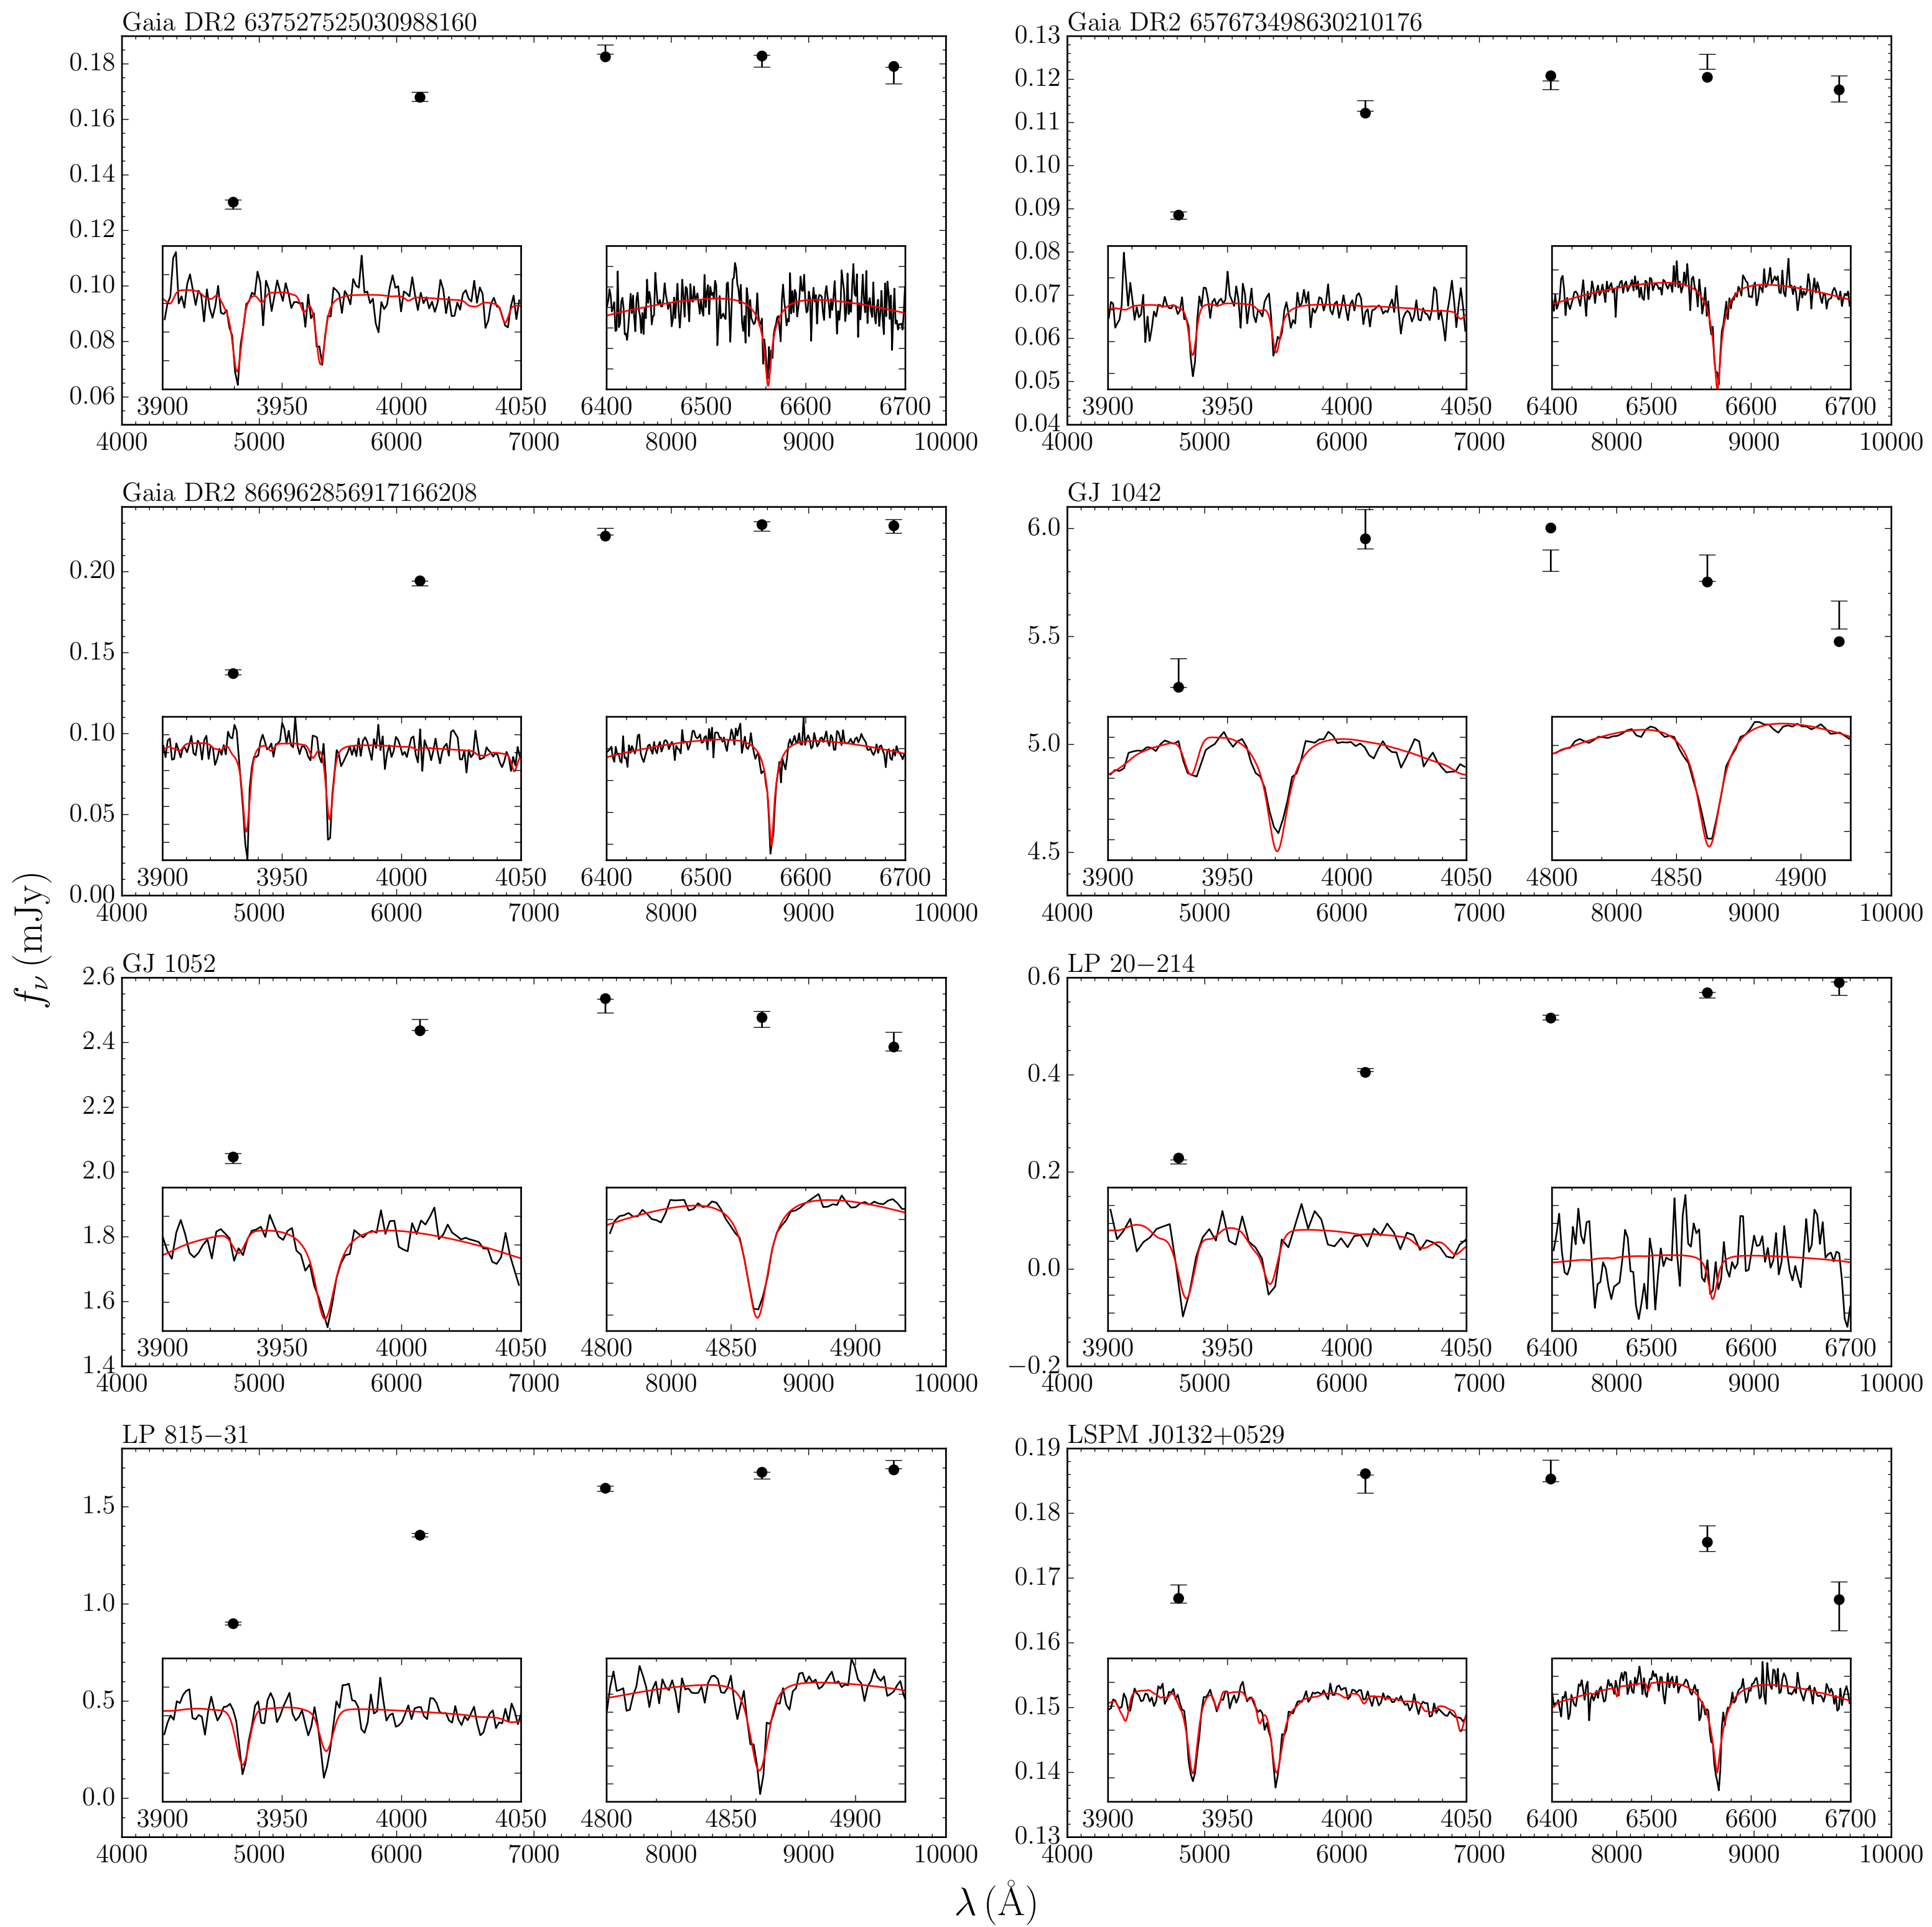

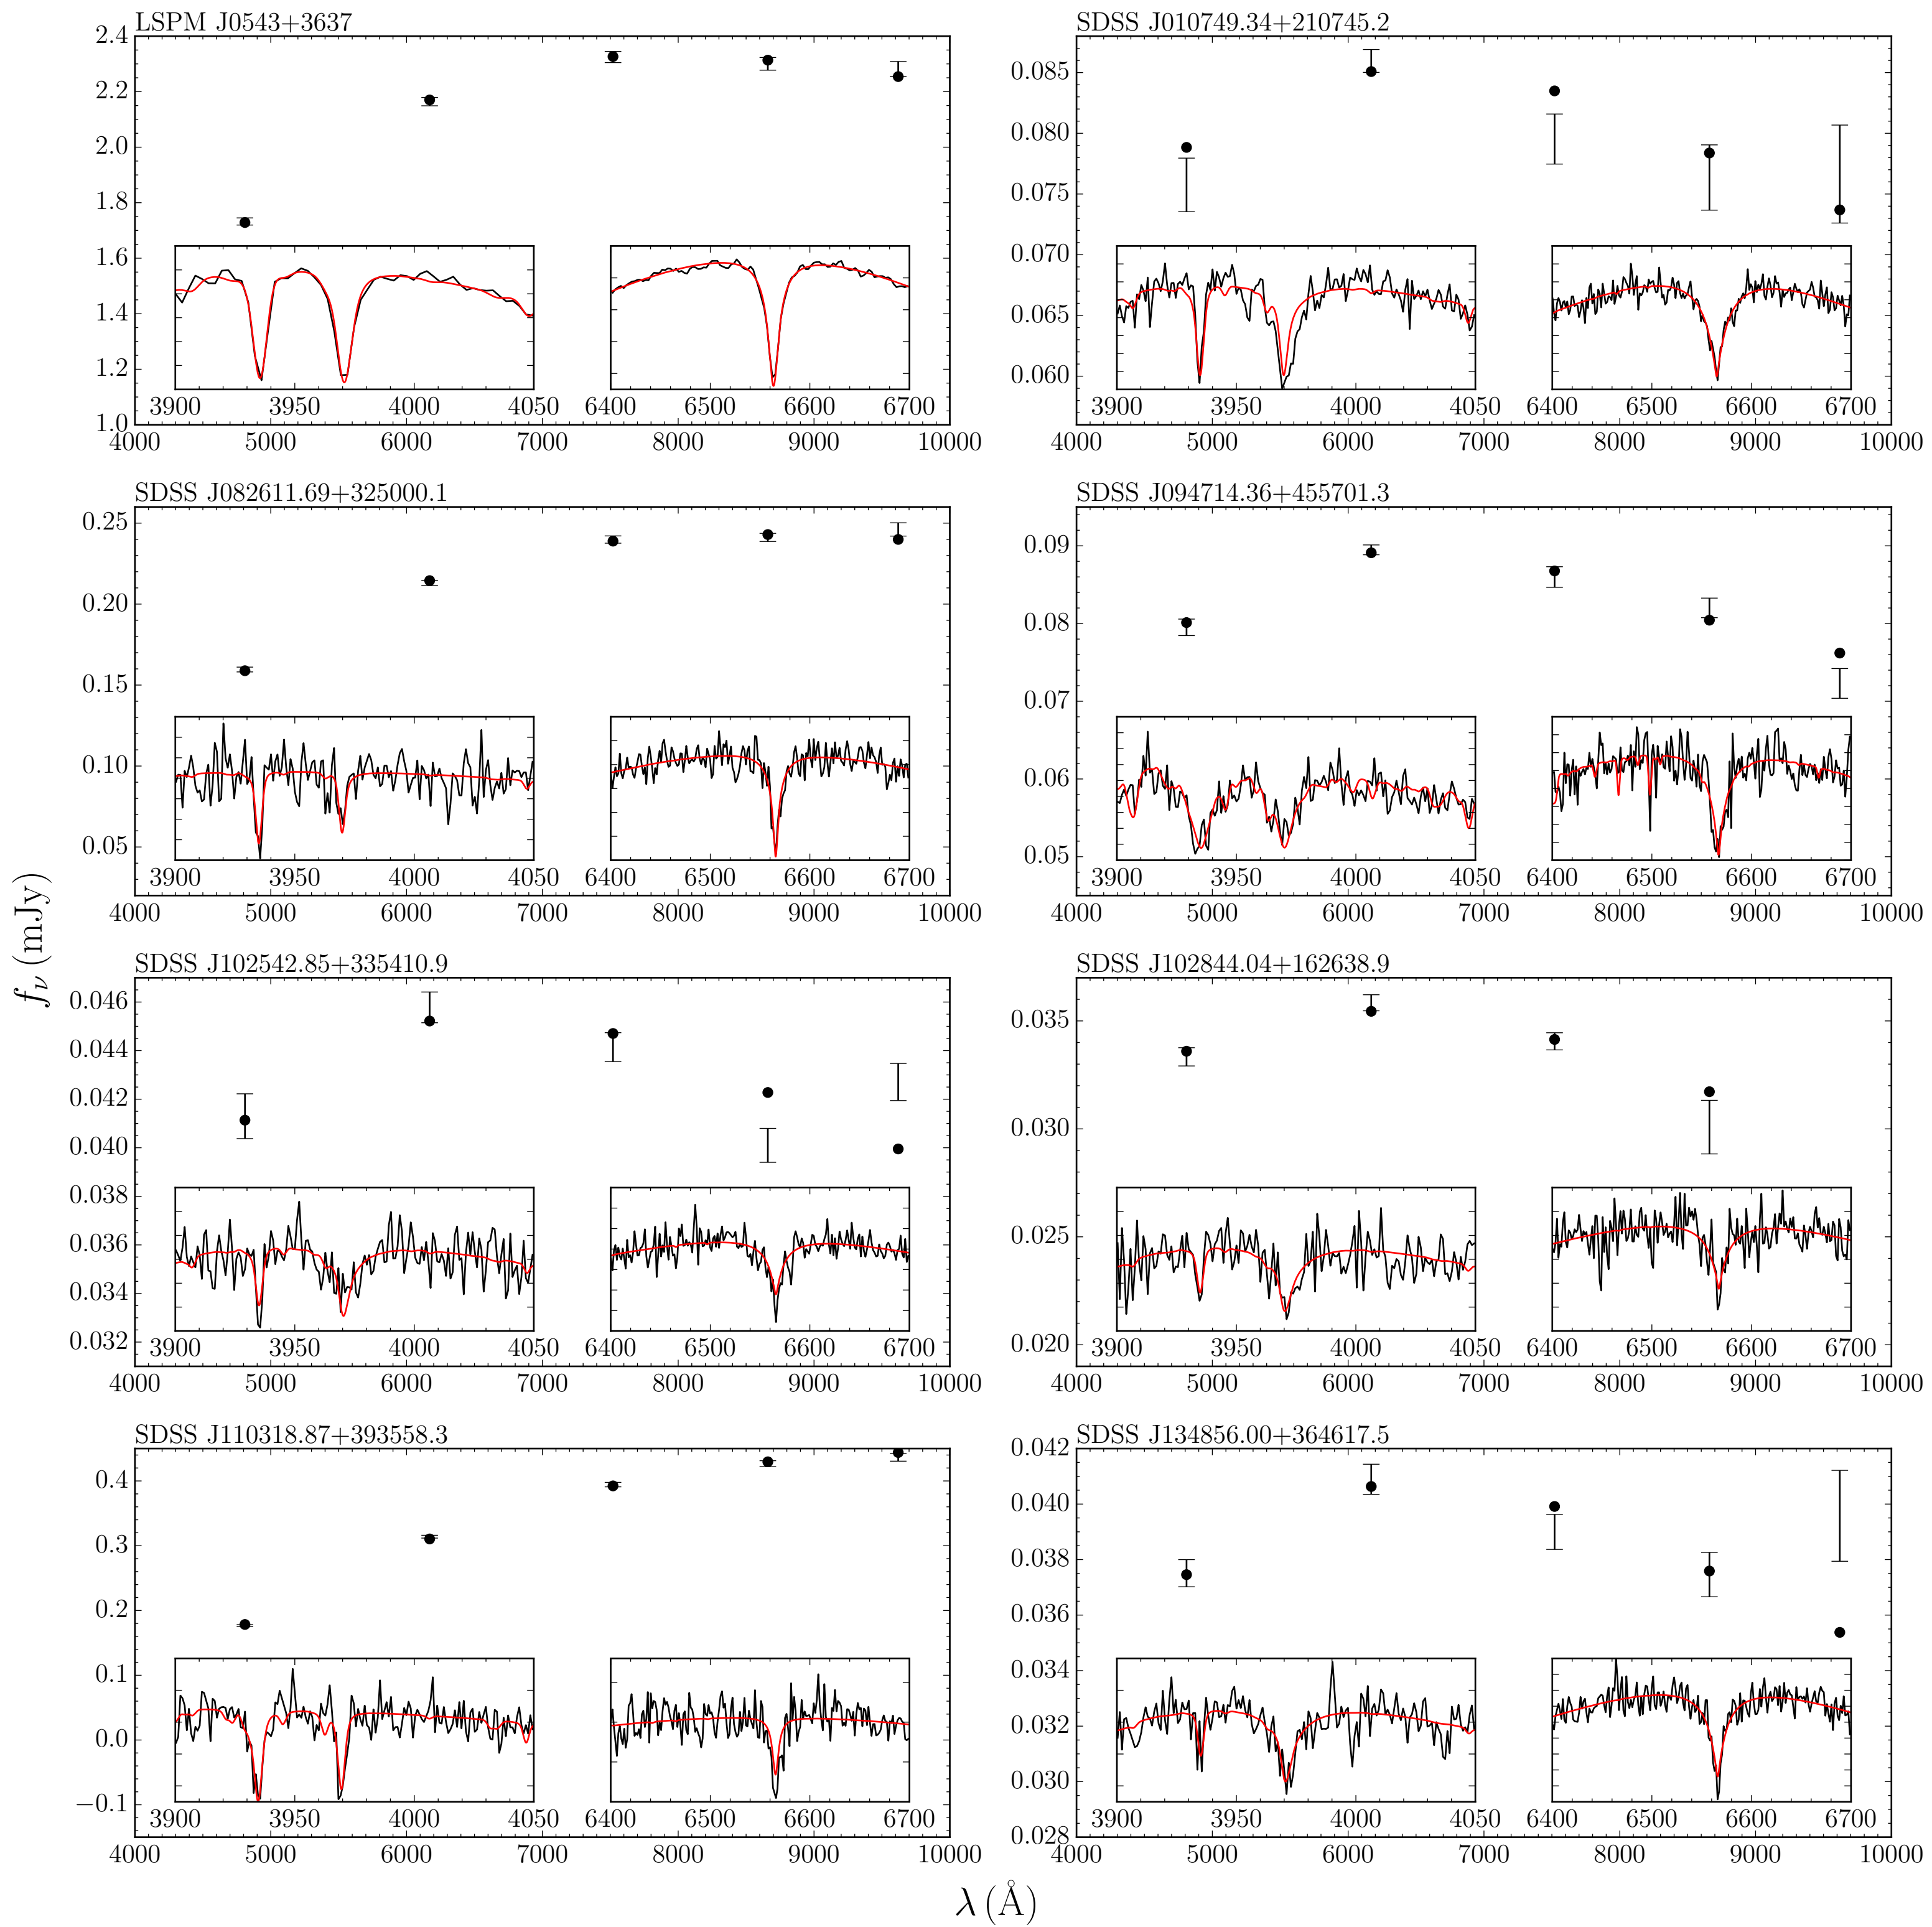

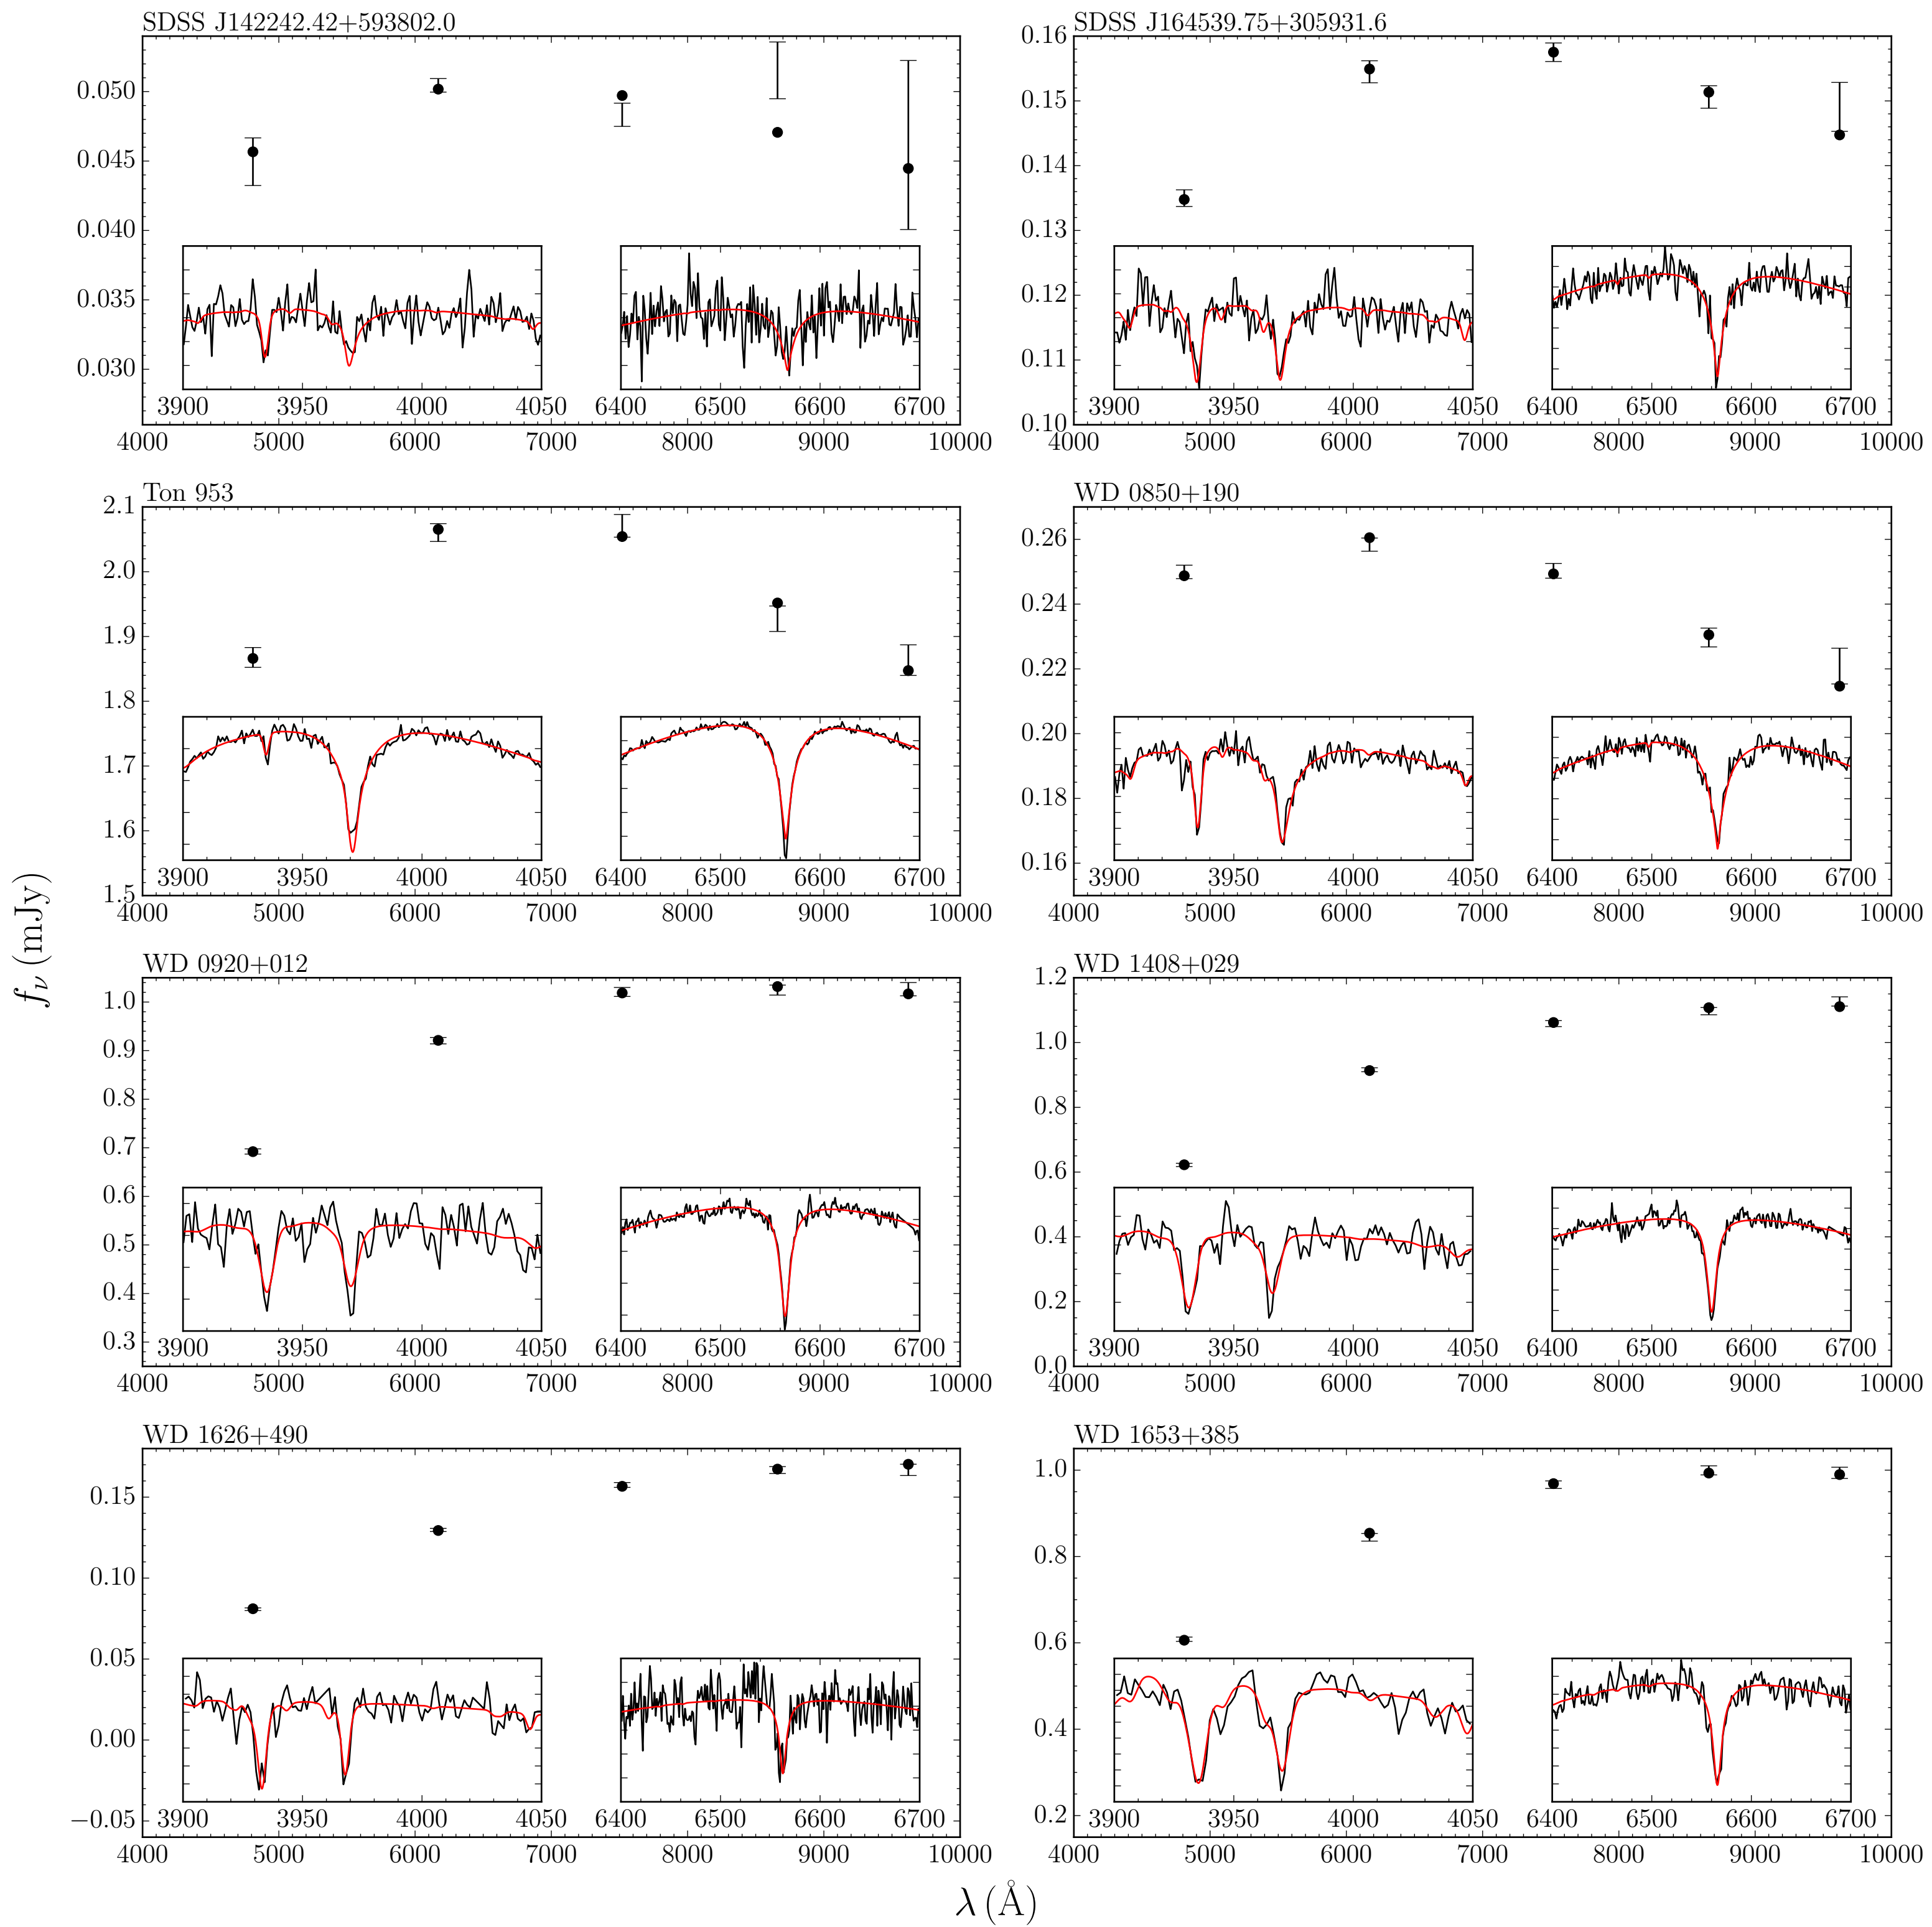

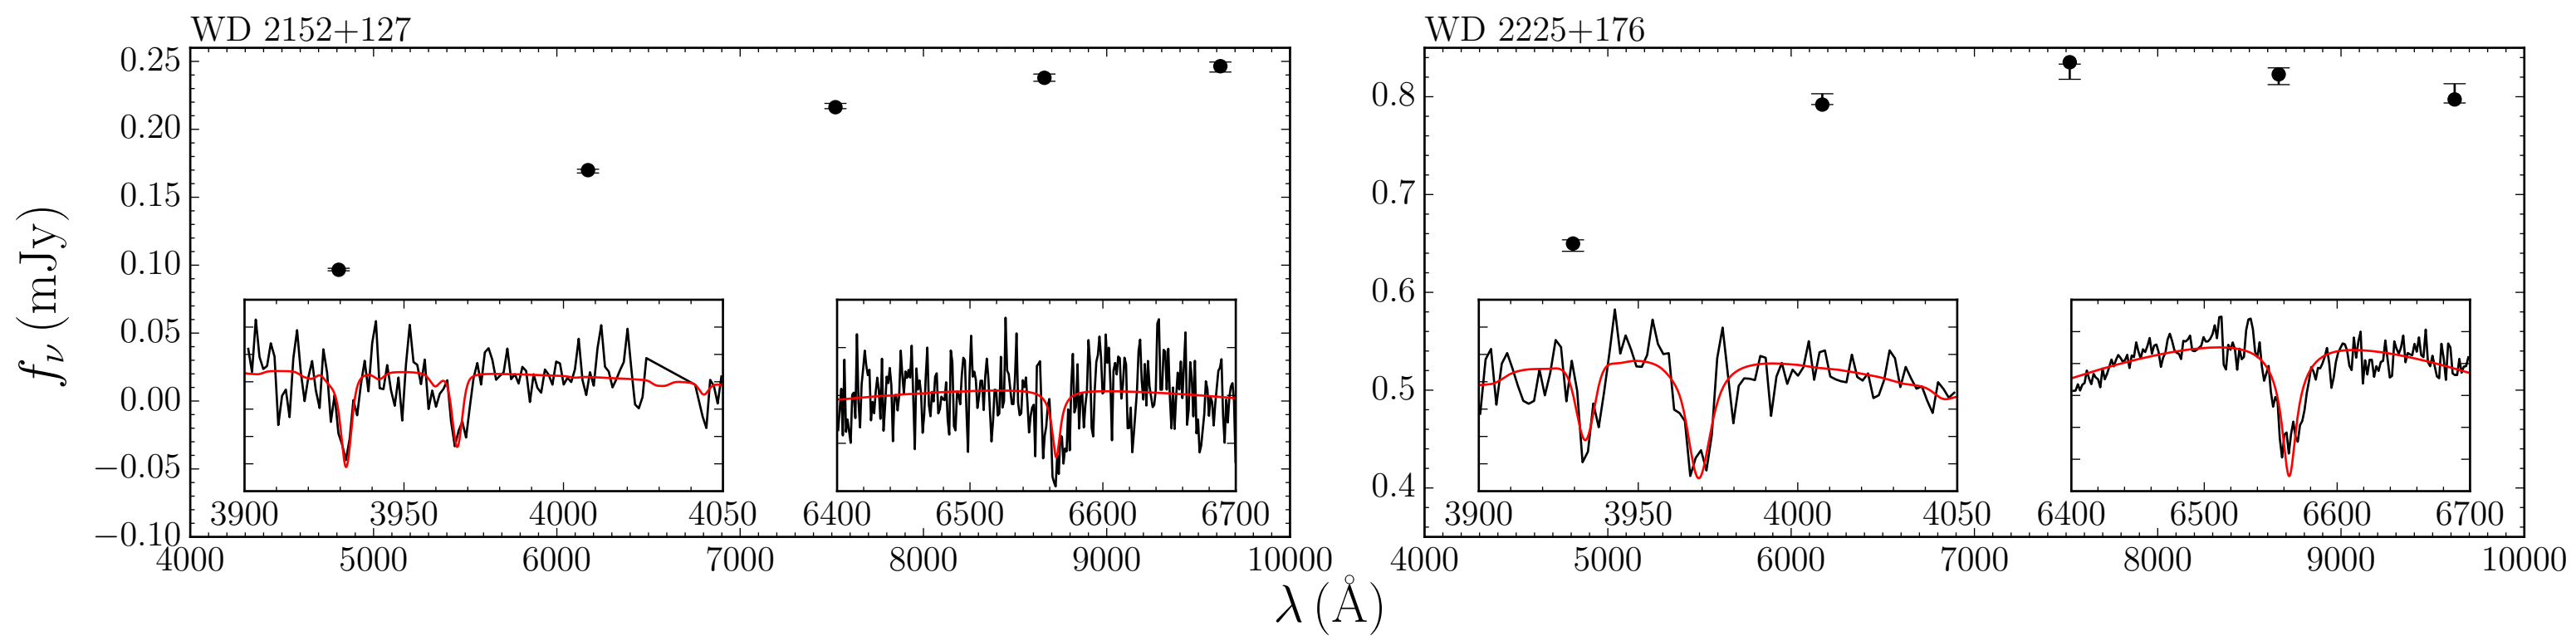

Supplement: Supplementary file 1 [file figure2_extended.pdf]
